# Supplementary material for: Real-time Network Intrusion Detection via Decision Transformers
Source: arXiv:2312.07696 source file (2023-12-17)
Supplement: Supplementary file 1 [file appendix.tex]

\newpage
\appendix
\onecolumn
\section{Theoritical Content}
